# Supplementary material for: Soccer on Your Tabletop
Source: arXiv:1806.00890 source file (2018-06-03)
Supplement: Supplementary file 1 [file G_Appendix.tex]

Intercepting the GPU calls between the video game engine and the graphics card using RenderDoc~\cite{renderdoc} usually results in a massive amount of information, from texture and depth buffers to blend shape weights of the participating human models. While it is easy to locate and extract the color/depth buffers, the other information is more difficult to parse. For example, the naming of the intercepted variables is not always meaningful and in order to use them more sophisticated methods are needed~\cite{Richter_2017}.

In our case, the area of action (soccer field) has specific dimensions and structure that can be used to infer information such as camera matrices. In particular, our goal is to estimate the video game camera modelview matrix $M_{\rm mv}$ and projection matrix $M_{\rm proj}$ 
(OpenGL/DirectX), so we can invert the depth buffer that it is in Normalized Device Coordinates (NDC). Below (Appendix~\ref{sec:appendix}) we describe the method to recover these matrices.
The additional information that we need is  a) a person segmentation of the texture buffer and b) an auxiliary camera that observes the field in world coordinates. 
To find which pixels belong to the players we use the semantic segmentation network of~\cite{Yu2015MultiScaleCA}. Then, for the auxiliary camera we follow the same approach as in Sec. 4.1: we estimate a camera with parameters $M_{aux}$ that observes the soccer field that lies in the world center with $y$ axis 0.  
Note that the intrinsics and extrinsics of the auxiliary camera cannot be used directly for estimating $M_{\rm proj}$ and $M_{\rm mv}$, since they do not include the near/far plane parameters and we do not know the video game's world system. 

\mysection{Estimating Video Game Cameras}{appendix}

To estimate the camera parameters (modelview and projection matrices) of a video game image, we need its corresponding NDC buffer, the auxiliary camera $M_{aux}$ that observes the field and the player segmentation mask.

The modelview and projection matrices in OpenGL/DirectX are $4\times4$ and the parameters to be estimated are the rotation vector $\theta_x, theta_y, theta_z$, the translation vector $t_x, t_y, t_z$ and focal length, near and far plane $f, z_{\rm near}, z_{\rm far}$.

Essentially we want to find the parameters that transformed the world scene to NDC so we can invert them:
\begin{equation}
\icol{x_{\rm clip}\\y_{\rm clip}\\z_{\rm clip}\\w_{\rm clip}} = M_{\rm proj} \, M_{\rm mv} \icol{x_{\rm world}\\y_{\rm world}\\z_{\rm world}\\1}
\end{equation}
\begin{equation}
\icol{x_{\rm NDC}\\y_{\rm NDC}\\z_{\rm NDC}} = \icol{x_{\rm clip}/w_{\rm clip}\\y_{\rm clip}/w_{\rm clip}\\z_{\rm clip}/w_{\rm clip}}
\end{equation}
To estimate the OpenGL cameras we can rely on the structure of the scene: points that belong to the soccer field (and not to players) should lie on a plane with $y$ equals to 0. The 3D world position of the ground pixels can be found by intersecting the rays from the auxiliary camera's ground pixels towards the ground. 
However, if we optimize only for the ground pixels, the $z_{\rm near}, z_{\rm far}$ parameters collapse, resulting in wrong reconstructions for the players. In addition to the ground constraint, we can minimize the reprojection error of the player 3D points to the auxiliary camera. 

Therefore, for a sets of world 3D points $X_p$ with $p\in ground$ and a set of 2D points (pixel location) $y_q$ with $q \in player$, the modelview matrix $M_{\rm mv}$ and the projection matrix $M{\rm proj}$ are found by minimizing:
\begin{equation}
\min \sum_{p \in {\rm ground}}(||X_p-\hat{X}_{p}||^2) + \lambda \sum_{q \in {\rm player}} (||y_q-\hat{y}_{q}||^2)
\end{equation}
with
\begin{align*}
\hat{X}_{p} = M_{\rm mv}^{-1} \, M_{\rm proj}^{-1} \, X_p^{\rm NDC},\\
\hat{y}_{q} = M_{aux} M_{\rm mv}^{-1} \, M_{\rm proj}^{-1} \, X_q^{\rm NDC}
\end{align*}

$X_p^{\rm NDC}$ and $X_q^{\rm NDC}$ correspond to the NDC coordinates of ground points $p$ and player points $q$. The NDC coordinates are found by dividing the the $x$ and $y$ pixel locations with image width and height respectively; the $z$ coordinate is the value of the depth buffer at the specific pixel location. The weight $\lambda$ was set to 0.01.

\section{Implementation Details}
\paragraph{Training Data} Our training data comes from the video game Electronic Arts FIFA 2016. The GPU calls between the game engine and the graphics card were obtained using RenderDoc v0.34. The playing teams were randomly selected and the camera was set to broadcast.

\paragraph{Player Analysis} Detection and pose estimation was performed using the code of \cite{Ren2015} and \cite{Wei2016ConvolutionalPM} respectively. Since the boxes can be lifted in 3D, very small or very large detections were removed. For tracking, two tracks were merged if the distance between them is less than 50 pixels and they are inside a frame window of 10 frames. 

We observed that a multi-person pose estimator better separates the players than bounding box overlap and it enables a simple algorithm for tracking. The pose estimation skeleton is also used for pixel-wise instance segmentation. In experiments with heavily occluded players, we found the pose estimator was significantly better in separating the occluded players than \cite{li2016fully} ($94\%$ vs $65\%$ in finding the correct number of players)

\begin{wrapfigure}{r}{3cm}
\hspace{-20px}
\includegraphics[width=0.2\textwidth]{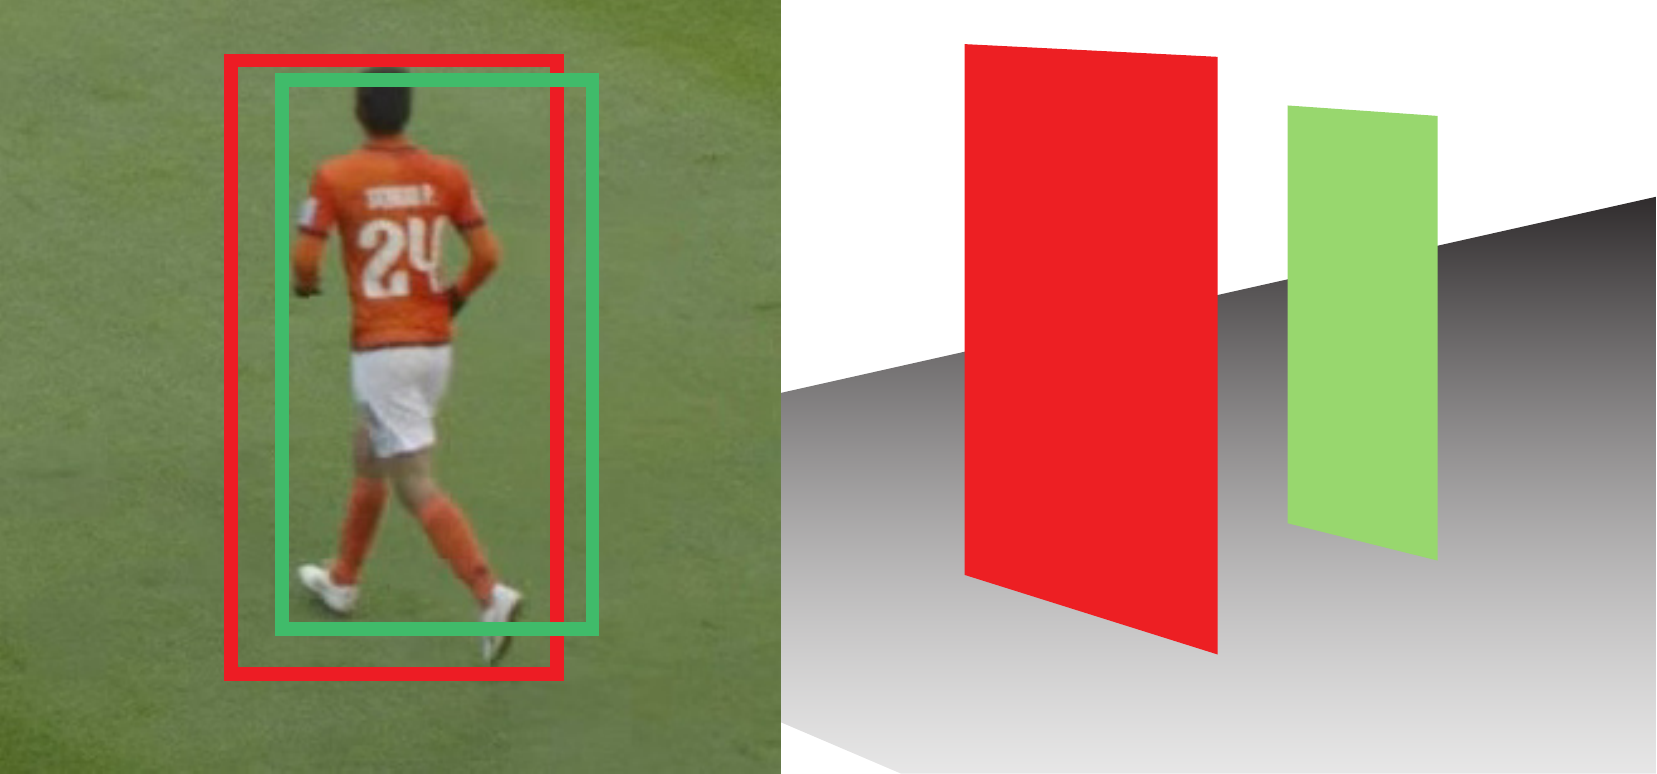}
\end{wrapfigure}
Tracking is used for temporal smoothing in 3D, removing jitter, and improving player segmentation.
The player mesh is generated from the estimated depth map and the player's 3D bounding box. 
Small errors in calibration or in the 2D bounding box (the green box shown here is a few pixels off) result in jittering of the 3D box (the assumption is that the bottom of the box lies on the ground) which is corrected using 3D temporal smoothing.

\paragraph{Ball Reconstruction}
\begin{wrapfigure}{r}{3cm}
\hspace{-20px}
\includegraphics[width=0.2\textwidth]{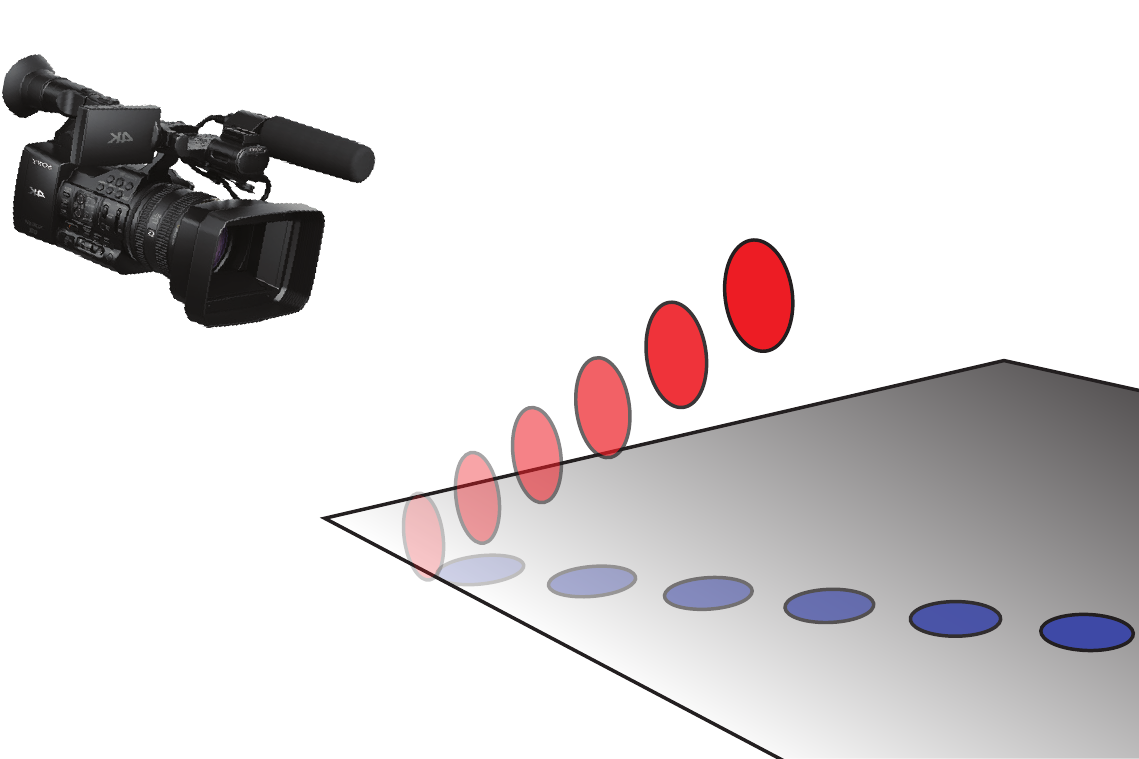}
\end{wrapfigure}
Our method does not reconstruct the 3D position of the ball (in some videos the ball was added manually). Our input is a monocular video and even with perfect 2D tracking of the ball, there is still ambiguity in the 3D ball trajectory that generated the 2D track. For example, we cannot disambiguate whether the ball is airborne moving straight away from the camera (red) or just moving in a straight line on the ground (blue), without incorporating ball physics (an area of future work).

\paragraph{Depth Estimation Network}
We used the Pytorch implementation of Stacked the Hourglass network~\cite{Newell2016StackedHN} with 8 stacks of 1 module. We performed optimization with the Adam solver with 0.0001 learning rate, 0.003 weight decay and betas were set to 0.9 and 0.999. Batch size was set to 6. The network was trained for 300 epochs with cross entropy loss.

We experimented with a number of network architectures: encoder-decoder with skip connections, fully convolutional with upsampling, and others, and we found that the hourglass model had superior performance. 

\paragraph{Scene Reconstruction}
The Soccer Hologram results were obtained using the Microsoft HoloLens Unity SDK and the capture of the video and images were performed using the Mixed Reality Capture from the HoloLens device. The varying-viewpoint results were obtained using Blender, where the reconstructed players were placed in a synthetic stadium with predefined camera paths. No user intervention was required for the players animation.
